# Supplementary material for: Automated approaches for band gap mapping in STEM-EELS
Source: arXiv:1705.00342 ancillary file (2018-10-18)
Supplement: Supplementary file 1 [file Supplementary.pdf]

# Supplementary Information

## Automated approaches for band gap mapping in STEM-EELS

*Cecilie S. Granerød, Wei Zhan, and Øystein Prytz*

*Department of Physics, Centre for Materials Science and Nanotechnology,*
*University of Oslo, P. O. Box 1048 Blindern, N-0316 Oslo, Norway*

### SI.1 Error bar mapping

The error bars calculated from the reduction in $R^2$ were used for evaluating single spectra in order to find the optimal fit parameter. However, when analyzing a Spectrum Image with several spectra, these error bars are also accessible for each analyzed spectrum, so that a map of the error associated with the onset can be created. The error is asymmetrically distributed around the onset, typically with a larger error to the low-end side. This originates from the fact that onset fitting is a one-sided fit where band gap fittings may have the tendency of resulting in a lower onset. Thus, low-end and high-end errors are not necessarily equal. Here, both ends of the error can be extracted separately in order to get more information about the fit accuracy, and correlations between onset, spectrum, and error can be found.

With the onset mapping shown in Fig. S1A, the corresponding total error (high-end error plus low-end error) is shown in Fig. S1B. Here the error is larger in ZnCdO than in ZnO, and there are some variations in the error in ZnCdO layer. This correlation is most likely caused by changes in the sharpness of the onset with varying Cd-content and band gap, where a sharper edge allows for a more accurate onset determination, leading to smaller error bars.

The variation in error bars can be seen to originate mostly from the low-end error, as seen in Fig. S1C, whereas the high-end error in Fig. S1D does not show the same variation. Fig. 1F shows a histogram of the error bars, where it is clear that the error is asymmetric: the high-end and low-end errors are not at the same values.

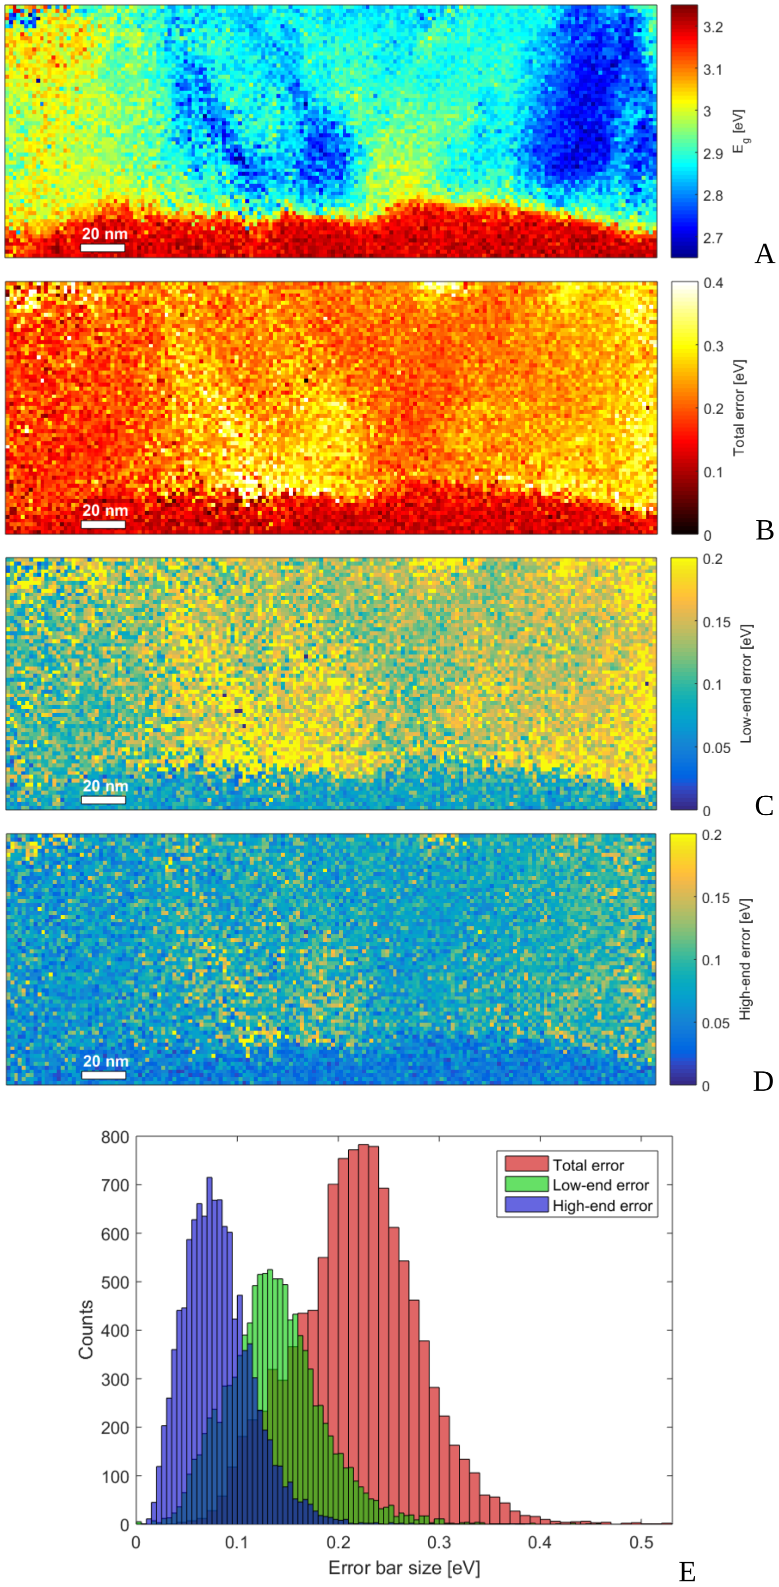


Fig S1: (A) Onset mapping; (B) Error from interpolated decrease of 0.05 in $R^2$; (C) Low-end of error; (D) High-end of error; and (E) Histogram of low-end, high-end and total error

## SI.2 Thickness correlation with band gap

It is known that the thickness of the TEM sample may affect the onset extraction, as a thicker sample gives a higher probability of generating Cherenkov radiation, typically leading to losses within the region of the band gap [1,2]. The thickness $t$ of the sample is often given in terms of the mean free path $\lambda$ of the electrons traveling through the material, and can be found from the ratio between the intensity within the zero-loss peak and the energy-loss spectrum [3].

The low loss spectrum is usually dominated by the plasmon peak, and obtaining this peak in the spectrum is crucial when performing thickness measurements in EELS. However, as the plasmons usually occur in the range of 15-25 eV (~19 eV for ZnO), a rather coarse dispersion needs to be used, while in the data sets analyzed in the current work, an experiment was set up with a dispersion of 0.01 eV per channel, to achieve the required accuracy in band gap onset extraction. The range of the acquisitions was therefore not sufficient to include the plasmon peak for thickness determination. However, assuming constant beam current throughout the experiment, an alternative approach is to use the intensity in the zero-loss peak to map thickness variations in the investigated regions. Although this method does not give in absolute or relative values for the thickness, it is assumed to be sufficient in order to pinpoint the thinner and thicker regions in the scanned area.

In each spectrum forming the onset map in Fig. S2A, the zero-loss was summed in an area up to 2.5 eV, as shown in Fig. S2C. The "thickness" mapping is shown in Fig. S2B, where it is clear that there are some thickness differences in the film. It can be seen that there is a gradual thinning towards one of the corners, which does not show in the mapping. Thus, there is very little correlation with thickness, as shown in the ZLP intensity versus onset in Fig. S2D. It could be that the Cherenkov radiation losses are sufficiently suppressed, or that the effects of these small losses are avoided in the fitting procedure.

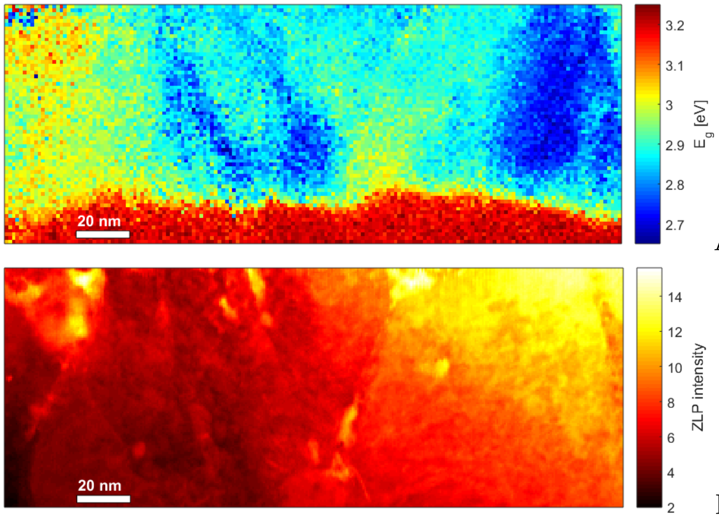


A

B

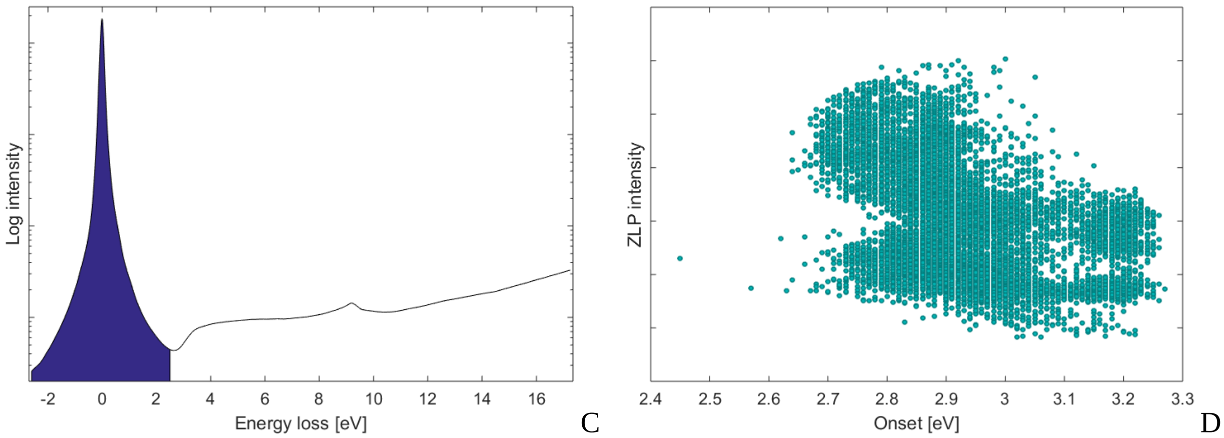


Fig S2: (A) Onset mapping; (B) ZLP intensity mapping; (C) ZLP intensity in spectrum; (D) Correlation between onset and ZLP intensity

## References


[1] L. Gu, V. Srot, W. Sigle, C. Koch, P. van Aken, F. Scholz, S.B. Thapa, C. Kirchner, M. Jetter, M. Rühle, Phys. Rev. B **75** (2007) 195214.

[2] M. Stöger-Pollach, P. Schattschneider, Ultramicroscopy **107** (2007) 1178.

[3] R.F. Egerton, Electron Energy-Loss Spectroscopy in the Electron Microscope, Springer US, 1986.
